# Supplementary material for: HypoML: Visual Analysis for Hypothesis-based Evaluation of Machine Learning Models
Source: arXiv:2002.05271 ancillary file (2020-02-12)
Supplement: Supplementary file 1 [file ReviewsFeedback.pdf]

# HypoML: Visual Analysis for Hypothesis-based Evaluation of Machine Learning Models

Qianwen Wang, William Alexander, Jack Pegg, Huamin Qu, and Min Chen

12 February 2020

## 1. Authors' Introduction

This article was submitted to EuroVis 2020 on 5 December 2020. It was not accepted. We appreciate the reviews provided by EuroVis 2020. Because the reviews have not identified any technical problems that would undermine the novelty and validity of this work, we think that the article is ready to be released as an arXiv report (after a few typo corrections), while we are seeking another opportunity for a formal publication. The following three sections are organized in reverse chronological order. We received the four reviews (Section 4) on 26 January 2020, and provided our short feedback (Section 3) on 30 January 2020. We received the summary review (Section 2) on 11 February 2020, together with the final decision.

## 2. EuroVis 2020 Summary Review

The reviewers each provided detailed reviews about the strengths and weaknesses of this submission. Each reviewer participated in the discussion. The primary concerns of the reviewers are summarized below, with strengths and additional details provided in the individual reviews.

- concerns for overall hypothesis-based approach (R1)
- limited contribution to the visualization literature (R2)
- concerns about choice of use case (R3,R2)
- technical soundness of all proposed inference rules (R1,R4)
- user evaluation may be required to test the effectiveness of the proposed method (R3)

## 3. Author Feedback (max ≤ 2000 characters) after receiving the Reviews (Section 4)

We thank the reviewers for their effort & comments. We hope once the following concerns are clarified, this novel VA work can be seen theoretically sound & practically useful.

R1R3[Complexity] The complexity is inherent in ML testing. Once we can test  $R(M,D)$  vs  $R(M+,D+)$ , we can make other 5 comparisons, which can provide some insight to model developers (MDs). Without VA, MDs cannot navigate the complexity of the analysis. This is maybe why no one formulated such tests before. Knowing VIS can help MDs, we identified all 12 hypotheses related to the 6 tests & derived the logical reasoning between the stats and hypotheses.

R2[Role of VA] VA(Vis+stats+logic) provides a solution to the complexity and enables rapid observation of the testing results.

R1[Mere debugging tool] Yes, but this is important & VA can help ML. If it were an NN method, it would not be for EuroVis.

R4[Prior work] We designed the tests in 2018 & did the logic in 2019. The 2nd & 3rd authors are ML specialists. The other three co-authors have strong VA+ML background.

R1[Hypothesis tests (HTs) are for small samples, not for large data tests in ML] a) Statistical significance depends on the entropy of the data space. Controlled studies in psychology have small samples for low-entropy spaces. ML has large samples for high-entropy spaces. HTs are meaningful to both. b) HTs are not for ensuring 100% correct.

R1[High threshold] We used  $P_t=0.05$  in all tests. Fig. 6 was intended to show that the threshold can be changed, though it would be better to show  $P_t=0.01$ . Comparing with other commonly used measures, eg, accuracy, precision, recall, F1, ..., thresholds for p-values are more standardised.

R1[1-tailed t-test] One can use 1-tailed here & it yields lower p-values. Textbook advice: use 2-tailed to show p-value.

R1[H9-H12] We defined this clearly in Sec 3 (last para.).

R2[Visual encoding] Vis is for showing the flow of reasoning, not the details of the logic. Splitting Vis into 3 views is not good.

## 4. EuroVis 2020 Reviews

### Reviews of 1052 HypoML: Visual Analysis for Hypothesis-based Evaluation of Machine Learning Models

Reviewer 4 (coordinator)

Paper Type

Algorithm / Technique

### **Scope (relevance to the event)**

Core topic, fits well

### **Contribution I (novelty, originality)**

This paper presents a method for model developers to test hypotheses about whether or not a feature is important, useful, or even learned by a model. The tool (HypeML) allows this rapid inference-based workflow. This situates the paper broadly into the important class of papers that try to ensure that people can understand and interpret models, as well as ensure some sense of fairness or other quality-focused metrics about their process/outcome.

### **Contribution II (novelty, originality)**

Strong: a strong contribution, clearly fill a gap in the literature

### **References**

At large, all important references are included

### **Utility, Importance (relevance in general)**

Addresses a clear need

### **Soundness (technical soundness, soundness of approach)**

Approach is (technically) correct and well justified

### **Reproducibility**

Many issues discussed, but some important details left out

### **Presentation Quality**

Excellent: exposition is clear and writing flows well

### **Argumentation Overall Rating**

Overall, I lean positive on this paper. I find it is an important area, and this provides a useful datapoint towards the overall goal. I also think the points 1 and 2 above can be addressed within the timeline of the review cycle.

### **Expertise**

Knowledgeable

### **The Review**

The paper does a good job motivating the problem, and leading the reader through the vision of how the problem will be addressed. The concept of hypothesis-based inquiry into models seems reasonable for the user expertise and use cases described in the paper.

There are two areas where the paper can be improved:

#### **1. Interactive Hypothesis-based Querying**

It appears that the hypotheses (H1-H12) are pre-defined. What is missing is a rationale for why these hypotheses, or even why hypotheses cannot be constructed by users (or asked via some other input modality). Were these based on prior work

(taxonomy?) that shows they are complete for a domain or group of users? Were they based on an interview study (or some other design process) that resulted in them? More information about this design process would help explain this choice (including why users cannot just create their own).

#### **2. Improve readability of section 4**

Section 4 is difficult to read. I understand this may be in part to the logical and statistical formulations included, but I found myself having to read sections of it multiple times to understand the gist of what components of this do. I recommend a careful revision of this section to make it more approachable/readable.

### **Reviewer 1 (committee member)**

### **Paper Type**

Algorithm / Technique

### **Scope (relevance to the event)**

Core topic, fits well

### **Contribution I (novelty, originality)**

The main contributions of this work are:

1. A novel conceptual framework for probing black box supervised classification models, based on statistical hypothesis testing and inference rules for twelve higher-order hypotheses, which are proposed to shed light on the question whether additional information has a beneficial effect on classification accuracy.

2. A visual encoding of the results of the hypothesis tests and the proposed inference rules that supports their practical use.

3. An implementation of a tool based on 1 and 2, and a discussion of usage scenarios related to image classification.

### **Contribution II (novelty, originality)**

Minor: only incremental improvements over previous work

### **References**

At large, all important references are included

### **Utility, Importance (relevance in general)**

Case for utility not compelling

### **Soundness (technical soundness, soundness of approach)**

Fundamentally unsound (technical) approach

### **Reproducibility**

Everything critical is discussed

### **Presentation Quality**

Good: only minor typos and grammar problems

### **Argumentation Overall Rating**

Even though the overall area of trying to gain a better understanding of competing machine learning models is timely and relevant, and even though I liked the idea of investigating machine learning models in a hypothesis-driven manner, I have quite fundamental reservations concerning soundness and utility of the specific approach proposed here, in particular against the use of formal statistical hypothesis testing. I remain unconvinced that it will lead to valid and useful conclusions, both from a theoretical perspective and given the limited empirical evaluation.

## Expertise

Expert

### The Review

I find the proposed approach of probing a machine learning method by combining multiple hypothesis tests to be highly questionable in several respects:

First, take the example from Fig.1: Finding out about rotation invariance. There are several recent approaches that enforce this via specific neural network architectures. In such a case, the proposed framework becomes a mere debugging tool that can be used to check whether the model was correctly implemented. It is not even clear why a human should be involved in the analysis - an automated unit test might do the job.

In my opinion, the interesting case for visual analytics is the one in which we want to find out whether the invariant has been learned from the training data without crafting it into the architecture. However, in this case, it is obvious that we can never expect perfect invariance. Therefore, the question "Is the hypothesis of rotation invariance true?" becomes meaningless: Of course, it is false (in a strict sense) and we will be able to reject it given enough data. In my opinion, what we are truly interested in in such a scenario is to which extent (i.e., up to which residual variation) it holds, and possibly if one model is better than another in maintaining it (e.g., because it was trained on an augmented input). Conceptually, a hypothesis test is not a suitable tool to answer such a question - we should rather pick an approach that focuses on effect size instead of a binary "reject / cannot reject" answer.

In other words: The paper highlights the fact that hypothesis testing is widely used in fields such as psychology, healthcare etc. and suggests using that as a blueprint for analyzing machine learning models. I believe that part of the reason for its popularity in other fields is the fact that, in psychology or healthcare, it is usually difficult to acquire very large samples. This makes sure that we do not get "significant" results for small effect sizes. On the other hand, we can usually evaluate

machine learning models in an automated way on huge test datasets. In this case, even tiny deviations from the null hypothesis will lead to its rejection. This makes hypothesis testing a much less useful tool, since almost no interesting null hypothesis will be true "exactly" / 100%.

Second, if we still want to follow a hypothesis testing approach despite these concerns, we need to account for type I and type II errors. These are completely ignored in the proposed system. The user can manually tweak a threshold for the p value, without any apparent guidance. Consequently, the system will act as if all corresponding hypotheses can be rejected with certainty, and it will actively encourage drawing firm higher-order conclusions from combinations of them. I find this to be particularly egregious given the fact that the presented experiments use quite high thresholds ( $p \leq 0.1$  in Fig. 6) despite testing multiple hypotheses - in such a scenario, it is highly likely that we will see at least one null hypothesis rejected even if all of them should in fact be true. By glossing over this, I find that the proposed approach misleads its users, especially given that it gives the (false) impression of mathematical exactness by applying the formalism of hypothesis tests and formalizing inference rules as equations.

Moreover, the authors state that they perform "paired, two-tail t-tests" (p. 5). In a two-tailed test, deviations in both directions (positive and negative) are counted as evidence against the null hypothesis. This does not fit together with the subsequent higher-order reasoning, which differentiates between positive and negative deviations. To do so, we would require two one-sided tests, and would have to reduce the alpha threshold accordingly.

I doubt that all proposed inference rules are correct. In particular, H9-H12 assume that a model that is given two inputs (M, D) can be decomposed into a part that processes M, and an "extra" part that accounts for the additional input. It might be possible to make such a decomposition for some specific models, but I do not think a valid inference can be made about these parts when treating the model as a "black box". To learn about H9-H12, I believe one would actually have to compute the decomposition and experiment with it, whereas the proposed approach only considers the integral model.

Finally, formulating the 12 hypotheses introduces huge complexity that is difficult to navigate despite the visual aids provided by the system. The authors report no feedback from domain experts on whether that complexity is required or helpful. Personally, I expect that asking the simple question

"Does a model benefit from a specific additional input, does it not make any difference, or does it hurt?" - which is answered every day by machine learning practitioners, by inspecting usually quite small tables without the need for a dedicated visual tool - will be enough in almost all cases.

Typos:

p.3: the the developer

p.7: in particularly -&gt; in particular

Reviewer 2 (reviewer)

## Paper Type

System

## Scope (relevance to the event)

Core topic, fits well

## Contribution I (novelty, originality)

In this paper, the authors outline a framework for testing out concepts learned by machine learning models using visual analytics to interpret the resulting differences in mean performance of various conditions. This matches the authors' claimed contribution, except it is unclear whether visual analytics makes much difference in the interpretation of the resulting differences in mean.

## Contribution II (novelty, originality)

Minor: only incremental improvements over previous work

## References

At large, all important references are included

## Utility, Importance (relevance in general)

Addresses a clear need

## Soundness (technical soundness, soundness of approach)

Some concerns on correctness, some choices questionable

## Reproducibility

Everything critical is discussed

## Presentation Quality

Excellent: exposition is clear and writing flows well

## Argumentation Overall Rating

The paper is well-written and addresses a problem which is very common among machine learning engineers and has no clear solution. When reasoning about models and data, machine learning engineers often test out new concepts to understand the semantic qualities of their models, and they can use statistics to confirm or deny their hypotheses. The solution proposed by the authors, a visualization of the results of six different analyses run on the ML model's

predictions under 4 different conditions, doesn't offer enough contribution to visualization research. Much of the paper is spent discussing experimental logic, which does communicate why reasoning about the results of such experiments is difficult. However, that doesn't translate into the discovery of effective visual encodings to deal with those difficulties.

## Expertise

Knowledgeable

## The Review

In this work, the authors present a visual analytics framework and system to test whether machine learning models are able to learn semantic concepts. Their framework requires a dataset that has been augmented with examples of this concept, and then runs the model under four conditions and conducts six types of analyses to test twelve hypotheses that are relevant to evaluating the semantic concept being studied. This is a well-thought out experimental methodology for the machine learning engineer to follow. The visualization proposed is clean and easy to understand, and the paper is very well written. However, the visual analytics solution proposed doesn't appear to help with the underlying task due to the simple visual encodings chosen. There is little contribution to the visualization literature. As an example of the visualization's short comings, the end of the introduction states that the VA tool was made because "model-developers may not be familiar with or remember the underlying statistical and logical analysis". The visual analytics tool should solve a more precise problem than that, and the accompanying use cases should demonstrate clearly that a problem is being solved by the visualizations that would not be easily solved without them.

## ## Technical Comments

- Need a better explanation of the sentence in section 3 that "there will always be some concepts that M cannot learn". Is this related to the finite number of constructs or dimensions? If they're infinite, we can learn all concepts?

- Concepts may be a bad term to use here - concepts and hypotheses are terms used in machine learning theory to represent potential models in the model space. I don't know if the term overloading is intentional by the authors. It's probably ok for this audience, but I wonder if it would make it hard for ML audiences to understand.

- At the end of section 3, the description of H9-12 is clunky because of the term "part". Can you provide an example here or describe in some clearer way?

- The concept is sound for experimental methodology, but the visualization has some issues. The histograms for each concept are too small to be useful. It's also unclear what visual effect is expected by laying out the analyses in rows - Do you expect patterns to emerge for users? The bipartite graph between histograms and the forest plot is difficult to read in its current format. In addition, the horizontal axis of the visualization is overloaded - on the left side of the visualization, it stands for analyses, and on the right side, it stands for results. Similarly, the vertical axis is overloaded. The visualization should really be demarcated into two parts.

- The visual encoding relies on reading small text that is often indiscernible (like discerning between  $R(M, D+)$  and  $R(M, D)$ ), and reasoning between several different parts of the visualization (H7 is supported by the third analysis which is then related to the model results 1 and 4). To me, when drilling down to look at one particular result of the analysis, it doesn't ease the cognitive load over something like figure 5, or a more regular statistical print out.

- In general, while the 12 hypotheses are related to the differences in model results, the visual encodings chosen don't help those relationships pop out for the sake of analysis. The visualization doesn't add to the effect of the overview of results.

- Both the overview and the drill down visual effects could be improved by some better visual encodings. For example,  $M$  and  $M+$  and  $D$  and  $D+$  would both be better represented by glyphs that made use of visual channels (maybe shapes with colors encoding whether it was the regular or the + condition).

- In the description of the visual encodings used, it is suggested that the experimental results (Figure 6c) is a novel choice. It is not; this is a standard forest plot that is widely used to communicate odds ratios in logistic regression models.

- The data augmentation used in the example is confusing to me, especially in Figure 7. Are you creating new images with both the regular version of the input image and a rotated version, but scaled down by  $1/4$ ? Because the concept itself isn't a contribution of your work, it would be better if you just used an exact example from the ML literature and cited the work that had a rotation transformer. You don't want to spend so much space on the methods of your experiment if the methods are not a contribution. It takes away from the generality of your framework.

- In general, the use case is too convoluted to provide clear support for your technique. First, it begins with a discussion about adding extra layers

to a CNN, which is not explored later. Second, there are too many tests and results and not enough analysis. You need a more gradual evaluation. Before going right to CNNs, run an experiment where we know what the results should be, and confirm to the reader that your system works in a proof of concept. An example could be classification between two gaussian clusters that overlap completely in one dimension but are separated in the second dimension. Treat the second dimension like extra data, and show that your system picks it out. If that's too simplistic, think of something more gradual than going right into CNNs, because the average reader may not know what results to expect out of the use case.

#### ## Style Comments

- Figure 2 - the last sentence is redundant. You also should have a sentence at the beginning of the caption explaining what the figure is showing (what is gradient ascent, at a high level). Also, is this your figure, or does it come from SDBR14? The attribution is unclear.

- You should be careful about conflating methods designed for computer vision tasks vs. methods designed for general machine learning. One example is in the related works paragraph starting with "In addition, researchers proposed techniques to summarize...", you might want to add at the end of that sentence, "especially in computer vision models."

- The subcaptions in Figure 3 are redundant since they are given in the text. I would use the space to give a better full caption to Figure 3. Consider that some readers go through the figures of a paper before deciding if they want to read it in full. What do you want them to take away from this figure?

- In figure 1, it looks like your classification model requires both the rotated bag and the unrotated bag to make a single prediction. That is confusing. Also, in the caption for fig 1, "One" is capitalized incorrectly. "Hypothese", in the visualization, is not pluralized correctly.

#### ## Typographical Errors

- "as shown by a recently establish ontology" => "established ontology"

#### ## Missing references

Should mention this paper by Adebayo et al about why saliency based methods may not be reliable.

Adebayo, Julius, et al. "Sanity checks for saliency maps." Advances in Neural Information Processing Systems. 2018.

[Reviewer 3 \(reviewer\)](#)

**Paper Type**

Algorithm / Technique

### Scope (relevance to the event)

Core topic, fits well

### Contribution I (novelty, originality)

The paper introduces HypoML, a visualization tool for testing a number of hypotheses about a machine learning (ML) model. The method relies on a user to formulate a hypothesis, e.g., that a particular data augmentation would improve the performance of the ML model. Under the proposed structured testing method, the user formulates 12 hypotheses for the comparison between the two models (with and without data augmentation) and uses HypoML to visualize the outcome of these comparisons as they relate to the 12 hypotheses.

The method seems overly complicated, and it is unclear how it improves well-established ML train-and-test frameworks. It is impossible to assess the value of the proposed method and tool because of a lack of user evaluation.

### Contribution II (novelty, originality)

Minor: only incremental improvements over previous work

### References

Some important references are missing

### Utility, Importance (relevance in general)

Case for utility not compelling

### Soundness (technical soundness, soundness of approach)

Some concerns on correctness, some choices questionable

### Reproducibility

Many issues discussed, but some important details left out

### Presentation Quality

Fair: some structural changes or some wordsmithing needed

### Argumentation Overall Rating

An overly complicated method, not clear how it improves existing ML workflows, and complete lack of user evaluation.

### Expertise

Expert

### The Review

The general idea of using hypothesis testing to evaluate ML models is interesting and worth exploring. The paper is well-written, and the authors try to appeal to the readers' intuition to explain the ideas. Unfortunately, the proposed method is overly complicated and hard to follow. It seems that existing train-and-test frameworks for

ML achieve most of the benefits of the proposed testing approach. Most importantly, the authors present no user evaluation of their method, making it impossible to judge how useful it is. For these reasons, I cannot recommend acceptance of the paper.

### Detailed comments

The proposed structured hypothesis testing method introduces a lot of complexity into the usual train-test-iterate development cycle for ML models. Section 4 "Statistical and Logical Reasoning of Hypotheses" was particularly difficult to follow. The authors fail to explain what this additional complexity achieves. The related work section needs to discuss existing train-and-test processes and tools in ML and statistics. How is the proposed process better than existing, well-established processes? Are users able to keep the complex interactions between hypotheses described in section 4 in mind?

It is not clear how the proposed hypothesis testing process relates to the visualizations in HypoML. Are the glyphs shown in Fig. 6 automatically updated by the system? How would the system be able to do this? The visualization using the matrix is also difficult to understand, especially how it relates to the process described in Section 4. For example, what exactly is shown in each column? The paper should describe these issues in more detail, and also give better justification for the design decisions.

The case studies described in Section 6 revolve around standard questions that come up in almost any ML model design. Experienced ML model builders know how to answer these questions using well-established train-and-test frameworks from the ML and statistical communities. It is unclear to me why one would need or use a more complex hypothesis testing framework in these standard scenarios. The authors should think of more complex scenarios where their framework could be applied, and then describe in detail how the proposed framework improves on existing methods.

Unfortunately, there is no user evaluation of the proposed hypothesis testing process or the HypoML tool. This makes it impossible to know if either of them is useful, and how they compare to standard processes and tools. For example, how would the proposed method compare to using TensorFlow and TensorBoard? The authors need to provide a detailed user study, both qualitative and quantitative, to demonstrate the effectiveness of their proposed method and tool.
